# Supplementary material for: BCS-BEC crossover in a $(t_{2g})^4$ Excitonic Magnet
Source: arXiv:2002.07351 source file (2020-02-18)
Supplement: Supplementary file 1 [file Supplemental_paper.pdf]

**SUPPLEMENTARY INFORMATION** for

# BCS-BEC crossover in a $(t_{2g})^4$ Excitonic Magnet

by N. Kaushal, R. Soni, A. Nocera, G. Alvarez, and E. Dagotto

## I. SPIN-ORBIT EXCITON OPERATORS IN THE $LS$ COUPLING LIMIT

Let us discuss first the spin-orbit exciton operators in the $LS$ coupling limit i.e. $(U >> t, \lambda)$. In the atomic limit, at $\lambda = 0$, the low-energy space has $L = 1$ and $S = 1$ with 9-fold degeneracy. The $(S = 0, L = 2)$ and $(S = 0, L = 0)$ states form higher energy manifolds located at energies $U/2$ and $5U/2$ (with respect to the ground state). In the limit of $U >> \lambda$, the $(S = 1, L = 1)$ manifold splits into $J_{eff} = 0$, 1, and 2 manifolds with degeneracies 1, 3, and 5. To investigate the action of our exciton operators in the strong coupling limit, below we write these exciton operators $(\Delta^{\dagger\tilde{j},m'}_{j,m})$ as a matrix spanned by the $J_{\rm eff} = 0$, 1, and 2 states of the $(S = 1, L = 1)$ manifold, where the states are denoted as $|m_{J_{\rm eff}}, J_{\rm eff}\rangle$:

$$\Delta^{\dagger\frac{3}{2},\frac{1}{2}}_{\frac{1}{2},\frac{1}{2}} = \begin{array}{c|ccccccccc} & |0,0\rangle & |\text{-}1,1\rangle & |0,1\rangle & |1,1\rangle & |\text{-}2,2\rangle & |\text{-}1,2\rangle & |0,2\rangle & |1,2\rangle & |2,2\rangle \\ \hline \langle 0,0| & 0 & 0 & -\frac{1}{2\sqrt{3}} & 0 & 0 & 0 & \frac{1}{6} & 0 & 0 \\ \langle \text{-}1,1| & 0 & 0 & 0 & 0 & 0 & 0 & 0 & 0 & 0 \\ \langle 0,1| & -\frac{1}{\sqrt{3}} & 0 & 0 & 0 & 0 & 0 & 0 & 0 & 0 \\ \langle 1,1| & 0 & 0 & 0 & 0 & 0 & 0 & 0 & 0 & 0 \\ \langle \text{-}2,2| & 0 & 0 & 0 & 0 & -\frac{\sqrt{2}}{3} & 0 & 0 & 0 & 0 \\ \langle \text{-}1,2| & 0 & 0 & 0 & 0 & 0 & 0 & 0 & 0 & 0 \\ \langle 0,2| & -\frac{1}{3} & 0 & -\frac{1}{\sqrt{6}} & 0 & 0 & 0 & \frac{1}{3\sqrt{2}} & 0 & 0 \\ \langle 1,2| & 0 & 0 & 0 & -\frac{1}{\sqrt{2}} & 0 & 0 & 0 & \frac{1}{3\sqrt{2}} & 0 \\ \langle 2,2| & 0 & 0 & 0 & 0 & 0 & 0 & 0 & 0 & 0 \end{array}$$

$$\Delta^{\dagger\frac{3}{2},\frac{-1}{2}}_{\frac{1}{2},\frac{-1}{2}} = \begin{array}{c|ccccccccc} & |0,0\rangle & |\text{-}1,1\rangle & |0,1\rangle & |1,1\rangle & |\text{-}2,2\rangle & |\text{-}1,2\rangle & |0,2\rangle & |1,2\rangle & |2,2\rangle \\ \hline \langle 0,0| & 0 & 0 & \frac{1}{2\sqrt{3}} & 0 & 0 & 0 & \frac{1}{6} & 0 & 0 \\ \langle \text{-}1,1| & 0 & 0 & 0 & 0 & 0 & 0 & 0 & 0 & 0 \\ \langle 0,1| & \frac{1}{\sqrt{3}} & 0 & 0 & 0 & 0 & 0 & 0 & 0 & 0 \\ \langle 1,1| & 0 & 0 & 0 & 0 & 0 & 0 & 0 & 0 & 0 \\ \langle \text{-}2,2| & 0 & 0 & 0 & 0 & 0 & 0 & 0 & 0 & 0 \\ \langle \text{-}1,2| & 0 & \frac{1}{\sqrt{2}} & 0 & 0 & 0 & \frac{1}{3\sqrt{2}} & 0 & 0 & 0 \\ \langle 0,2| & -\frac{1}{3} & 0 & \frac{1}{\sqrt{6}} & 0 & 0 & 0 & \frac{1}{3\sqrt{2}} & 0 & 0 \\ \langle 1,2| & 0 & 0 & 0 & 0 & 0 & 0 & 0 & 0 & 0 \\ \langle 2,2| & 0 & 0 & 0 & 0 & 0 & 0 & 0 & 0 & -\frac{\sqrt{2}}{3} \end{array}$$

$$\Delta^{\dagger\frac{3}{2},\frac{1}{2}}_{\frac{1}{2},\frac{-1}{2}} = \begin{array}{c|ccccccccc} & |0,0\rangle & |\text{-}1,1\rangle & |0,1\rangle & |1,1\rangle & |\text{-}2,2\rangle & |\text{-}1,2\rangle & |0,2\rangle & |1,2\rangle & |2,2\rangle \\ \hline \langle 0,0| & 0 & 0 & 0 & \frac{-1}{2\sqrt{6}} & 0 & 0 & 0 & \frac{-1}{2\sqrt{6}} & 0 \\ \langle \text{-}1,1| & \frac{-i}{\sqrt{6}} & 0 & 0 & 0 & 0 & 0 & 0 & 0 & 0 \\ \langle 0,1| & 0 & 0 & 0 & 0 & 0 & 0 & 0 & 0 & 0 \\ \langle 1,1| & 0 & 0 & 0 & 0 & 0 & 0 & 0 & 0 & 0 \\ \langle \text{-}2,2| & 0 & \frac{i}{\sqrt{2}} & 0 & 0 & 0 & \frac{i}{3\sqrt{2}} & 0 & 0 & 0 \\ \langle \text{-}1,2| & \frac{i}{\sqrt{6}} & 0 & 0 & 0 & 0 & 0 & 0 & 0 & 0 \\ \langle 0,2| & 0 & 0 & 0 & \frac{-1}{2\sqrt{3}} & 0 & 0 & 0 & \frac{-1}{2\sqrt{3}} & 0 \\ \langle 1,2| & 0 & 0 & 0 & 0 & 0 & 0 & 0 & 0 & \frac{-2}{3} \\ \langle 2,2| & 0 & 0 & 0 & 0 & 0 & 0 & 0 & 0 & 0 \end{array}$$

$$\Delta^{\dagger\frac{3}{2},\frac{-1}{2}}_{\frac{1}{2},\frac{1}{2}} = \begin{array}{c} \\ \langle\, 0,0| \\ \langle -1,1| \\ \langle\, 0,1| \\ \langle\, 1,1| \\ \langle -2,2| \\ \langle -1,2| \\ \langle\, 0,2| \\ \langle\, 1,2| \\ \langle\, 2,2| \end{array} \begin{array}{c} \begin{array}{ccccccccc} |0,0\rangle & |\text{-}1,1\rangle & |0,1\rangle & |1,1\rangle & |\text{-}2,2\rangle & |\text{-}1,2\rangle & |0,2\rangle & |1,2\rangle & |2,2\rangle \end{array} \\ \begin{bmatrix} 0 & \frac{i}{2\sqrt{6}} & 0 & 0 & 0 & \frac{-i}{2\sqrt{6}} & 0 & 0 & 0 \\ 0 & 0 & 0 & 0 & 0 & 0 & 0 & 0 & 0 \\ 0 & 0 & 0 & 0 & 0 & 0 & 0 & 0 & 0 \\ \frac{-1}{\sqrt{6}} & 0 & 0 & 0 & 0 & 0 & 0 & 0 & 0 \\ 0 & 0 & 0 & 0 & 0 & 0 & 0 & 0 & 0 \\ 0 & 0 & 0 & 0 & \frac{i\sqrt{2}}{3} & 0 & 0 & 0 & 0 \\ 0 & \frac{i}{2\sqrt{3}} & 0 & 0 & 0 & \frac{-i}{2\sqrt{3}} & 0 & 0 & 0 \\ \frac{-1}{\sqrt{6}} & 0 & 0 & 0 & 0 & 0 & 0 & 0 & 0 \\ 0 & 0 & 0 & \frac{-1}{\sqrt{2}} & 0 & 0 & 0 & \frac{1}{3\sqrt{2}} & 0 \end{bmatrix} \end{array}$$

Using the matrices shown above and the definitions of the Triplon operators as $\mathbf{T}^\dagger_n|0,0\rangle{=}|n,1\rangle$ and the Quintuplon operators as $\mathbf{Q}^\dagger_l|0,0\rangle{=}|l,2\rangle$, where $n \in \{0,\pm1\}$ and $l \in \{0,\pm1,\pm2\}$, then we can write that $\Delta^{\dagger 3/2,s/2}_{1/2,s/2}|0,0\rangle = (s\frac{\mathbf{T}^\dagger_0}{\sqrt{3}} - \frac{\mathbf{Q}^\dagger_0}{3})|0,0\rangle$, $\Delta^{\dagger 3/2,1/2}_{1/2,-1/2}|0,0\rangle = (-\iota\frac{\mathbf{T}^\dagger_{-1}}{\sqrt{6}} + \iota\frac{\mathbf{Q}^\dagger_{-1}}{\sqrt{6}})|0,0\rangle$, and $\Delta^{\dagger 3/2,-1/2}_{1/2,1/2}|0,0\rangle = (-\frac{\mathbf{T}^\dagger_1}{\sqrt{6}} - \frac{\mathbf{Q}^\dagger_1}{\sqrt{6}})|0,0\rangle$. The above equations show that these conventional electron-hole pair excitation operators when acting on the $|J_{\text{eff}} = 0\rangle$ ground state leads to local Triplon and Quintuplon excitations in the strong coupling limit, and this explains the presence of two bands in the exciton pair-pair susceptibility strong-coupling calculations shown in the main text.

## II. CONDENSATION OF EXCITONS IN THE TRIPLET CHANNEL

For the exciton $\Delta^{\dagger 3/2m'}_{1/2m}$, $m$ and $m'$ can take two values, $\{\pm1/2\}$, which leads to singlet and triplet channels for the condensation. We define the exciton operators in both channels as follows:

$$\phi_s(i) = \sum_m \Delta^{\dagger 3/2m}_{1/2m}(i), \tag{1}$$

$$\boldsymbol{\phi}_t(i) = \sum_m \Delta^{\dagger 3/2m}_{1/2m'}(i)\boldsymbol{\tau}_{mm'}. \tag{2}$$

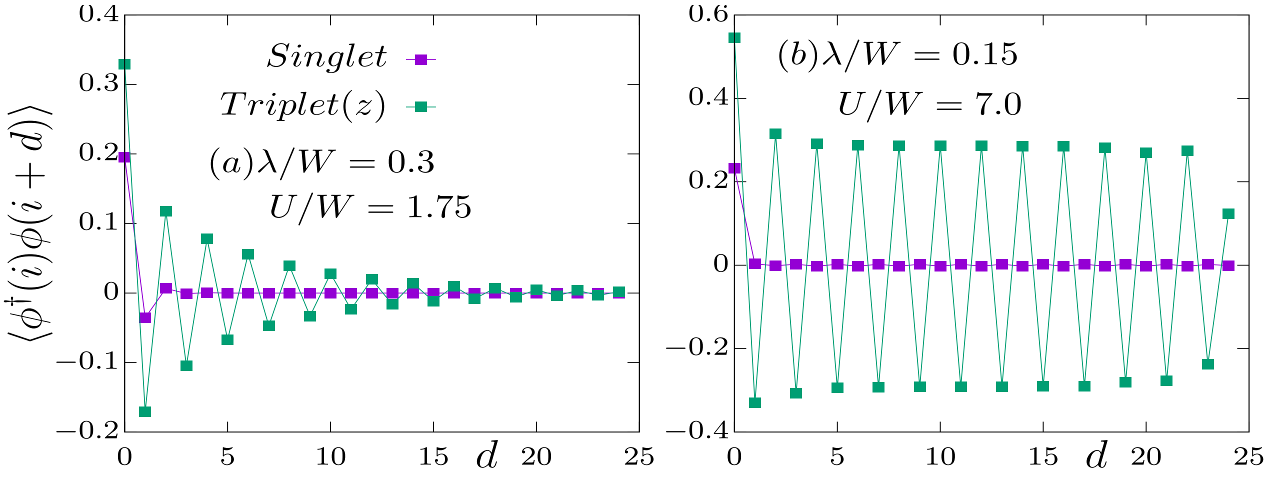


FIG. 1: Panels (a) and (b) show the exciton-exciton correlation in the singlet and the $z$-component of the triplet channels for the cases $(\lambda/W, U/W) = (0.3, 1.75)$ and $(0.15, 7.0)$, respectively. A system size $L = 32$ is used, and site $i = 8$ is fixed.

Figure 1 displays the excitonic correlation in the channels indicated in the caption, using a $L = 32$ sites chain, for the two $(\lambda/W, U/W)$ points chosen in the DMRG phase diagram corresponding to the BCS $(0.3, 1.75)$ and BEC

$(0.15, 7.0)$ regions. The correlations are measured with respect to the 8th-site from the left boundary. It is clear that the excitons condense in the triplet channel in both the BCS and BEC regimes. However, as concluded in the main text using the momentum distribution function of excitons, in the BCS regime the triplet local-exciton correlation decays fast with distance while it shows nearly long-range order characteristics in the BEC regime.

## III. DETAILS OF $A_{jm}(q, \omega)$ CALCULATIONS

We used the DMRG-correction vector target method to calculate the single-particle spectral function $A_{jm}(q, \omega - \mu)$. The chemical potential is calculated using $\mu = (E_{N+1} - E_{N-1})/2$, where $E_N$ is ground state energy of the $N$-particle system. The spectral function below and above $\mu$ is calculated using the following formulas, with a fixed broadening $\eta = 0.1$ eV:

$$A_{jm}(i, c, \omega < \mu) = -\frac{1}{\pi} Im[\langle \Psi_G | a^{\dagger}_{jm,i} \frac{1}{-\omega - H + E_G + \iota\eta} a_{jm,c} | \Psi_G \rangle], \tag{3}$$

$$A_{jm}(i, c, \omega > \mu) = -\frac{1}{\pi} Im[\langle \Psi_G | a_{jm,i} \frac{1}{\omega - H + E_G + \iota\eta} a^{\dagger}_{jm,c} | \Psi_G \rangle]. \tag{4}$$

In the equations above, $i$ and $c$ are sites. We fixed $c = L/2$ at the center, and calculated $A_{jm}(i, c, \omega)$ for all other sites $i$'s. Then, we employed the following approximation to reduce the computational cost:

$$A_{jm}(q, \omega) = \frac{1}{L} \sum_i e^{\iota(i-c)q} (A_{jm}(i, c, \omega < \mu) + A_{jm}(i, c, \omega > \mu)) \tag{5}$$

To calculate the density of states $\rho_{jm}(\omega)$, we used $\rho_{jm}(\omega) = A_{jm}(c, c, \omega < \mu) + A_{jm}(c, c, \omega > \mu)$.

To reproduce the data shown in this publication, the open source DMRG++ program and input files are available at *https://g1257.github.io/dmrgPlusPlus/*.
